# Supplementary material for: Structural roles and gender disparities in corruption networks
Source: arXiv:2504.17086 source file (2025-04-23)
Supplement: Supplementary file 1 [file supplementary.pdf]

# Structural roles and gender disparities in corruption networks

**Arthur A. B. Pessa[1], Alvaro F. Martins[1], Mônica V. Prates[1], Sebastian Gonçalves[2], Cristina Masoller[3], Matjaž Perc[4,5,6,7,8,*], and Haroldo V. Ribeiro[1,*]**

[1]Departamento de Física, Universidade Estadual de Maringá, Maringá, PR 87020-900, Brazil
[2]Instituto de Física, Universidade Federal do Rio Grande do Sul – Porto Alegre, RS 91501-970, Brazil
[3]Departament de Física, Universitat Politécnica de Catalunya, Rambla St. Nebridi 22, Terrassa, 08222, Barcelona, Spain
[4]Faculty of Natural Sciences and Mathematics, University of Maribor, Koroška cesta 160, 2000 Maribor, Slovenia
[5]Community Healthcare Center Dr. Adolf Drolc Maribor, Ulica talcev 9, 2000 Maribor, Slovenia
[6]Department of Physics, Kyung Hee University, 26 Kyungheedae-ro, Dongdaemun-gu, Seoul 02447, Republic of Korea
[7]Complexity Science Hub, Metternichgasse 8, 1030 Vienna, Austria
[8]University College, Korea University, 145 Anam-ro, Seongbuk-gu, Seoul 02841, Republic of Korea
[*]email: matjaz.perc@gmail.com, hvr@dfi.uem.br

## Supplemental Materials

**Table S1.** Hypothesis testing equality in the average values of network centralities of females and males for Brazilian and Spanish corruption networks via the bootstrap test. The table presents $p$-values for each centrality measure, for each country, and distinguishes between all nodes and recidivists. The null hypothesis of equal mean values is rejected at the 95% confidence level when $p < 0.05$.

| Centrality | Country | All males/females | Recidivist males/females |
|---|---|---|---|
| Degree | Brazil | 0.357 | 0.304 |
| Degree | Spain | 0.053 | 0.176 |
| Betweenness | Brazil | – | 0.321 |
| Betweenness | Spain | – | 0.549 |

**Table S2.** Hypothesis testing equality in distribution of network centralities of females and males for Brazilian and Spanish corruption networks via the Mann-Whitney test. The table presents $p$-values for each centrality measure, for each country, and distinguishes between all nodes and recidivists. The null hypothesis of equal centrality distributions is rejected at the 95% confidence level when $p < 0.05$.

| Centrality | Country | All males/females | Recidivist males/females |
|---|---|---|---|
| Degree | Brazil | 0.832 | – |
| Degree | Spain | 0.405 | 0.374 |
| Betweenness | Brazil | – | 0.104 |
| Betweenness | Spain | – | 0.211 |

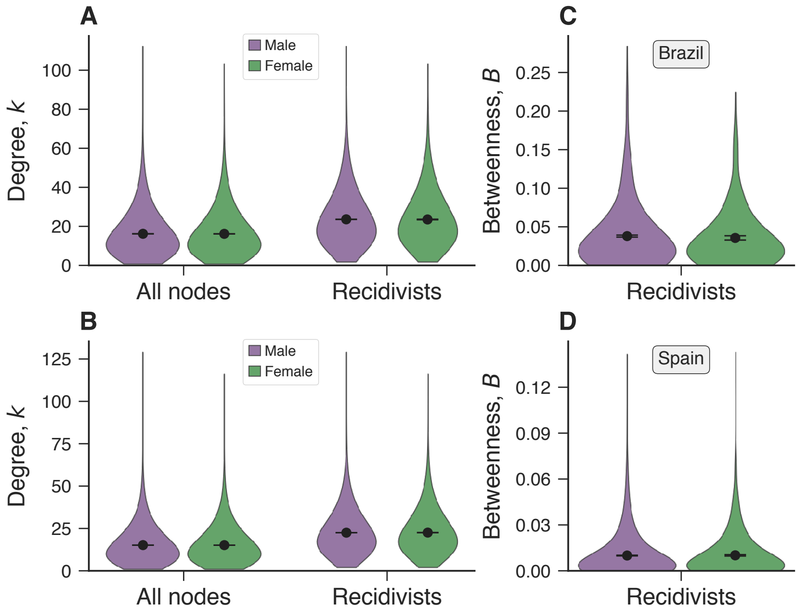


**Figure S1.** Network centralities of males and females in corruption networks simulated from our null model. Panels (A) and (B) show the degree centrality $k$ of males (purple) and females (green), with nodes further categorized into all agents and recidivists. Panels (C) and (D) show the betweenness centrality $B$ of recidivist agents. Results are based on 1,000 simulations of the null model, with parameters calibrated to Brazilian (top row) and Spanish (bottom row) data. Error bars indicate the mean centrality values and their standard errors. Violin plots illustrate the data distributions.

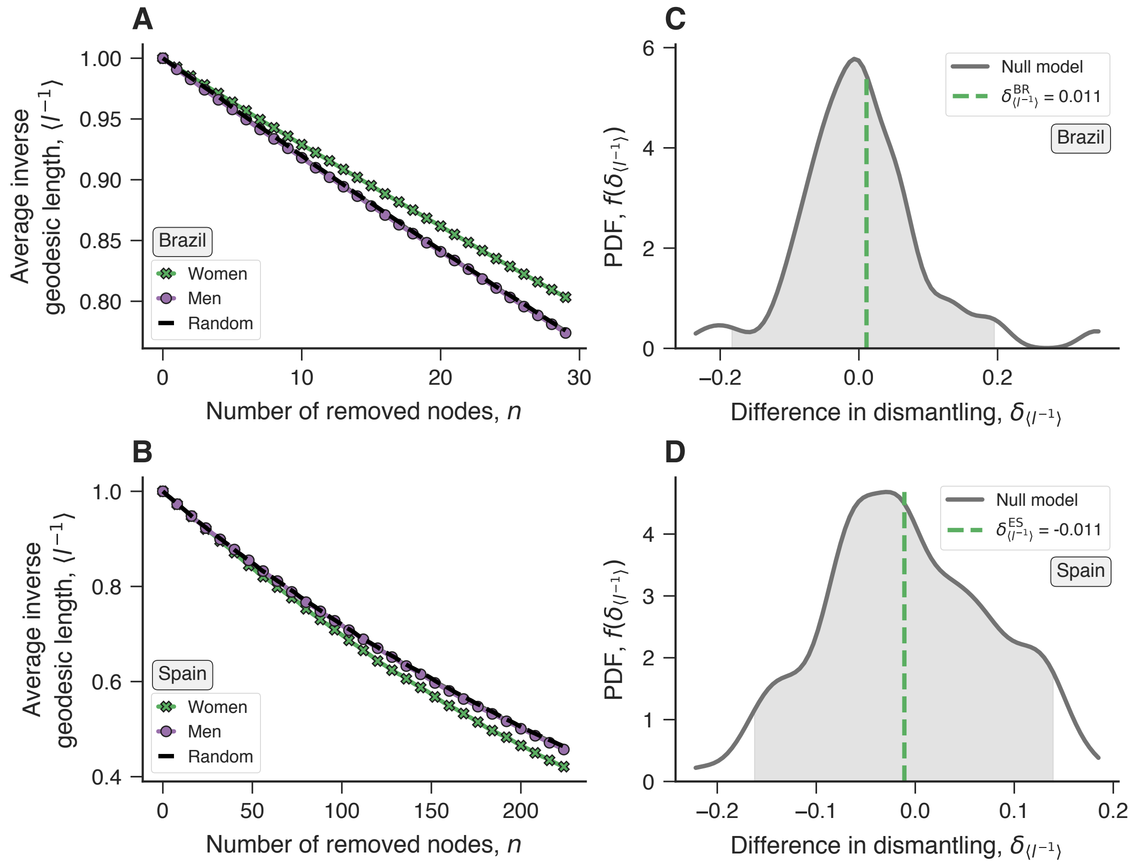


**Figure S2.** Network resilience under random removal of male and female agents as quantified by the average inverse shortest paths. Average value of the inverse shortest path length $\langle l^{-1} \rangle$ of the (A) Brazilian and (B) Spanish networks as a function of the number of removed nodes $n$ following three random dismantling strategies: randomly removing all females (green crosses), randomly removing the same number of males (purple circles), and randomly removing the same number of agents regardless of gender (dashed lines). The curves represent average values calculated from 1,000 independent realizations of each dismantling strategy. Probability distribution functions [PDFs, $f(\delta_{\langle l^{-1} \rangle})$] comparing the differences $\delta_{\langle l^{-1} \rangle}$ in the final values of the average inverse shortest paths after randomly removing females and randomly removing nodes regardless of gender in 1,000 simulations of networks generated from our null model for the (C) Brazilian and (D) Spanish networks. Empirical differences are indicated by vertical lines.

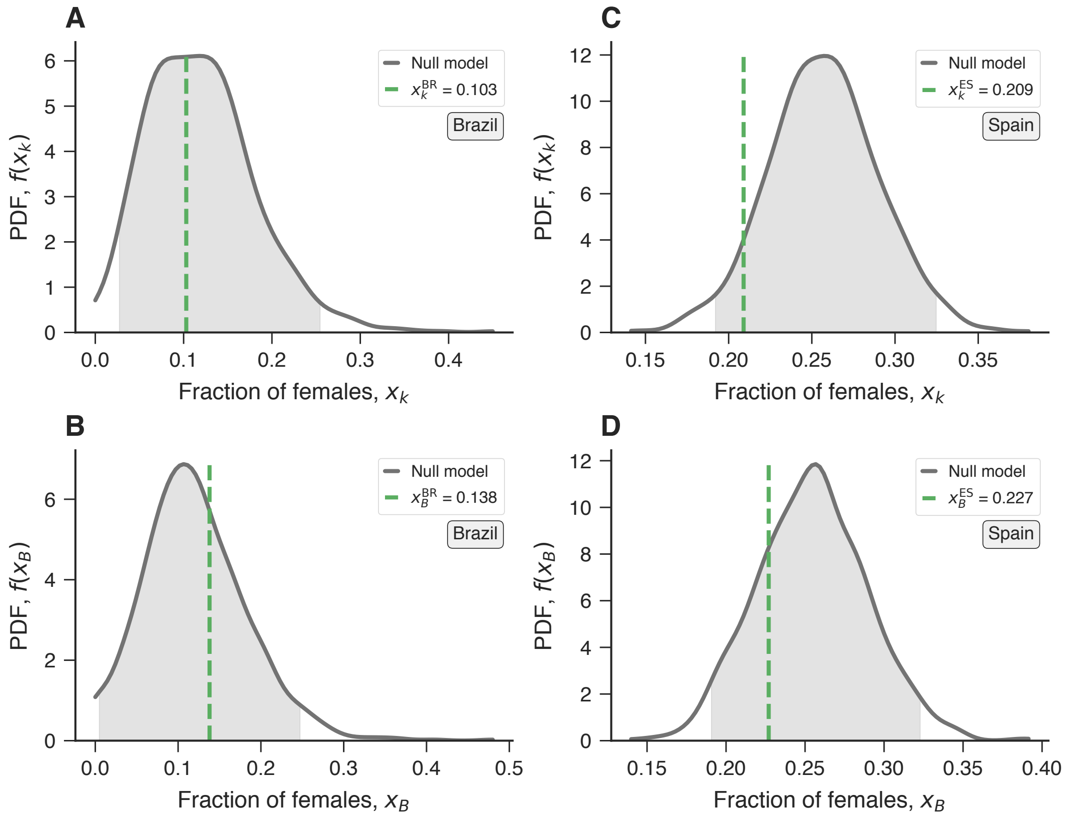


**Figure S3.** Fractions of females removed from corruption networks following dismantling strategies based on removing nodes with the highest degree and betweenness centrality. Probability distribution functions $[f(x), x \in (x_k, x_B)]$ of observing a fraction $x$ of female agents among the nodes selected for removal by decreasing values of degree [$x_k$, panels (A) and (B)] and betweenness [$x_B$, panels (C) and (D)] across 1,000 simulations of our null model for the Brazilian and Spanish corruption networks. Empirical fractions are depicted by vertical lines, with shaded regions corresponding to 95% confidence intervals estimated from the null model.

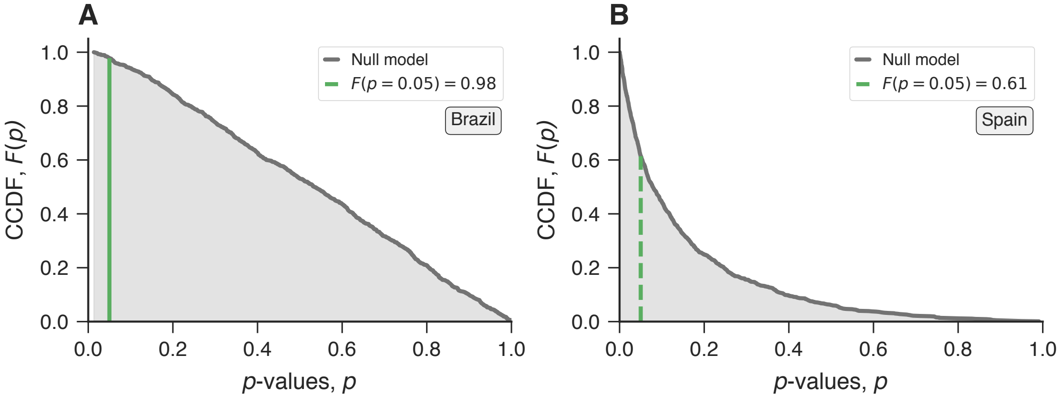


**Figure S4.** Comparison of the empirical fraction of females involved in corruption scandals with the null model simulations. Complementary cumulative distribution functions [CCDF, $F(p)$] of the $p$-values obtained by testing the equality in distribution of the fraction of females in the (A) Brazilian and (B) Spanish networks against each one of 1,000 null model simulations per network. The $p$-values refer to the Mann-Whitney test, with green vertical lines indicating the 95% confidence level ($p = 0.05$). The fractions of comparisons that do not reject the null hypotheses of equality in distribution [$F(p > 0.05)$] are shown with the panels.

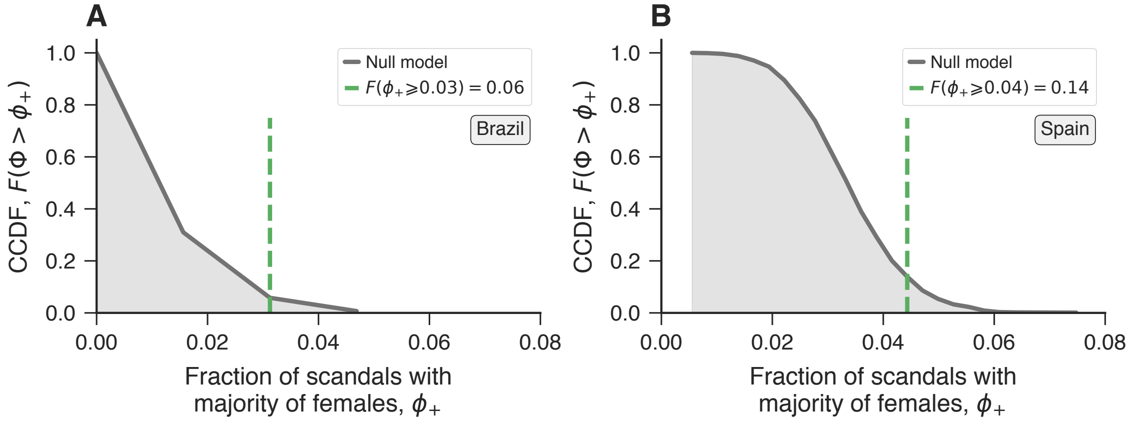


**Figure S5.** Fractions of scandals predominantly involving females obtained from null model simulations compared with their empirical counterparts. Complementary cumulative distribution functions [CCDF, $F(\phi_+)$] of the fraction of scandals predominantly involving females $\phi_+$ obtained from 1,000 null model simulations of (A) Brazilian and (B) Spanish networks. Empirical fractions are depicted by vertical lines with the probabilities of observing the same fractions in the null model shown with the panels.

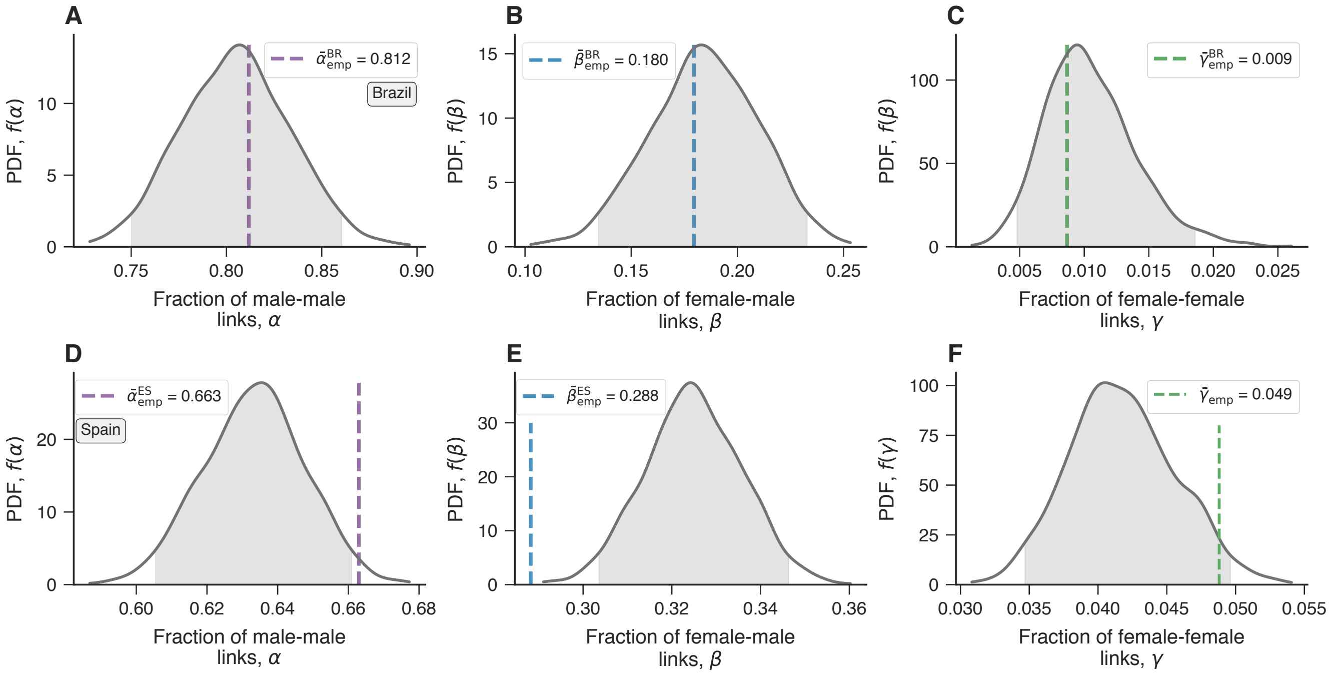


**Figure S6.** Fractions of male-male, female-male, and female-female links obtained from null model simulations compared with their empirical counterparts. Probability distribution functions [PDFs, $f(\cdot)$] of average fractions of links (A) exclusively between males $f(\alpha)$, (B) between males and females $f(\beta)$, and (C) exclusively between females $f(\gamma)$, obtained from 1,000 null model simulations of the Brazilian corruption network. Panels (D)-(F) display the corresponding distributions from 1,000 null model simulations of the Spanish corruption networks. Shaded areas represent 95% confidence intervals, with vertical lines indicating the empirical fractions of each link type.
